# Supplementary material for: Itinerancy enhanced quantum fluctuation of magnetic moments in iron-based superconductors
Source: arXiv:1503.02653 source file (2015-03-09)
Supplement: Supplementary file 1 [file supplementary_r2v1.pdf]

# Supplementary

This supplementary provides additional detailed information about our calculation that is based on well-established methods in the literature.

## I. Preparing for the 5-band Hamiltonian of the itinerant carriers

The figure below illustrates the overall computation scheme already outlined in the manuscript, involving several well-established methods.

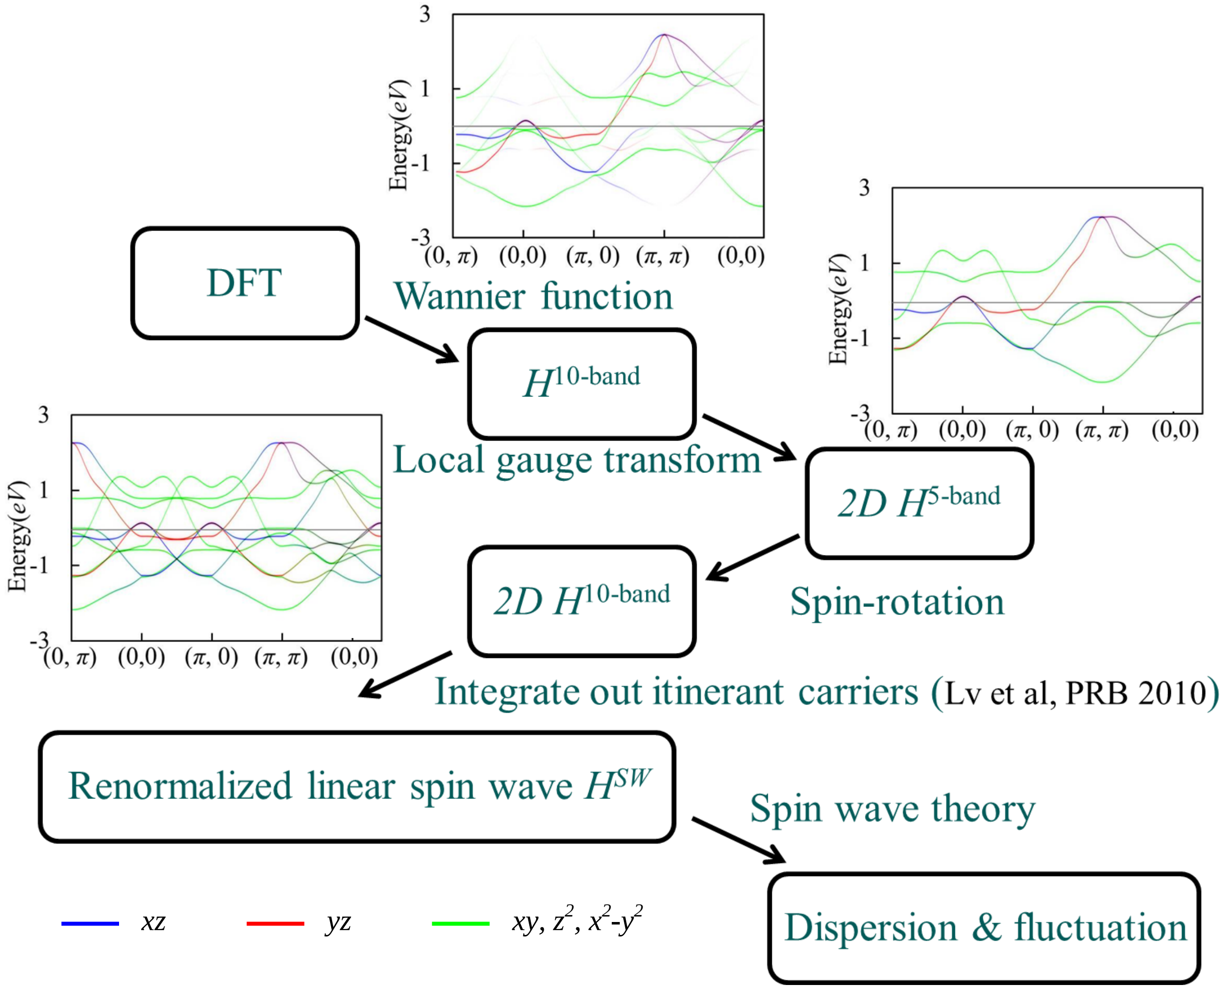


We start with a density functional theory calculation using the experimental lattice constant. We then construct the low-energy Wannier orbitals spanning the energy window of the Fe-*d* bands, and use them to represent the fully self-consistent Kohn-Sham Hamiltonian of the normal state. These steps have been reported previously [C.-C. Lee et al., PRL 103, 267001 (2009)]. The

resulting three-dimensional Hamiltonian contains 10 bands, because there are two Fe atoms in the unit cell due to the alternating tetrahedron positioning of the As atoms around each Fe atom. We then perform the local gauge transformation [Lee and Wen, Phys. Rev. B 78, 144517 (2008)] that changes the sign of the orbitals of even $z$-parity on the even lattice sites, to take into account the glide translational symmetry and recover a nearly translational symmetry Hamiltonian in the new "pseudo-momentum" space. Upon dropping the small out-of-plane terms, we finally obtain a translation symmetric two-dimensional 5-band Hamiltonian for the itinerant carriers. This final Hamiltonian corresponds to one Fe in the unit cell, and is thus consistent with the unit of local moments to be considered in the next step.

# II. Integrating out the itinerant carriers

Our goal is to study the influence of the itinerant carriers on dispersion and fluctuation of local moments. We thus follow the procedure reported in [Lv, el al. PRB 82, 045125 (2010)] to integrate out the itinerant carriers to obtain a effective linear spin-wave Hamiltonian. It is convenient to first perform a spin rotation for the site of even columns of sites $S_i^x = \tilde{S}_i^x$, $S_i^y = \kappa_i \tilde{S}_i^y$ and $S_i^z = \kappa_i \tilde{S}_i^z$, where $\kappa_i = \exp(\mathrm{i}\mathbf{Q}\cdot\boldsymbol{r}_i) = \pm 1$, and $\tilde{c}_{i,\uparrow} = c_{i,\downarrow}$, such that in the rotated frame, all the ordered local moments are pointing toward the "up" direction. Note that in this new frame, the itinerant Hamiltonian again resumes a 10-band form, since now spin up and spin down channels couple together after the spin rotation.

We then use the Holstein-Primakoff boson: $\tilde{S}_i^z = S - a_i^\dagger a_i$, $\tilde{S}_i^+ = \sqrt{2S} a_i$, $\tilde{S}_i^- = a_i^\dagger \sqrt{2S}$, to capture the bare spin-excitation of the local moment via the spin-wave Hamiltonian (in unit of $S^2$):

$$\mathcal{H}_{loc} = \sum_q [A_0(q)\left(a_q^\dagger a_q + a_{-q} a_{-q}^\dagger\right) + B_0(q)\left(a_q^\dagger a_{-q}^\dagger + a_{-q}\, a_q\right)] \qquad [1]$$

where,

$$A_0(q) = 2(J_1 cosq_y + 2J_2)/S$$

$$B_0(q) = 2(J_1 cosq_x + 2J_2 cosq_x cosq_y)/S$$

Treating the Hund's coupling between the itinerant and local degrees of freedom, $\frac{J_H}{2S}$, as perturbation

$$\mathcal{H}_H = -\frac{J_H}{2S} \sum_{i,\alpha,\nu\nu'} \boldsymbol{S}_i c_{i\alpha\nu}^\dagger \boldsymbol{\sigma}_{\nu\nu'} c_{i\alpha\nu'} \qquad [2]$$

where $\boldsymbol{\sigma}_{\nu\nu'} = (\boldsymbol{\sigma^x}, \boldsymbol{\sigma^y}, \boldsymbol{\sigma^z})_{\nu\nu'}$with $\boldsymbol{\sigma^\alpha}$, the canonically transformed full Hamiltonian (Eq.1 of the manuscript)

$$e^{\Delta}\mathcal{H}e^{-\Delta} = \mathcal{H} + [\Delta, \mathcal{H}] + \frac{1}{2}\left[\Delta, [\Delta, \mathcal{H}]\right] + \cdots \quad [3]$$

gives the renormalized linear spin-wave Hamiltonian from its quadratic components:

$$\mathcal{H}^{sw} = \mathcal{H}^{sw}_{loc} + \langle \mathcal{H}^2_H + \frac{1}{2}\left[\Delta, \mathcal{H}^{(1)}_H\right]\rangle_e = \sum_q [A(q)\left(a^\dagger_q a_q + a_{-q}a^\dagger_{-q}\right) + B(q)\left(a^\dagger_q a^\dagger_{-q} + a_{-q}\, a_q\right)] \quad [4]$$

up to 2nd order in 1/S, where

$$A(q) = A_0(q) + A_1 + A_2(q) \quad [5]$$

$$B(q) = B_0(q) + B_2(q) \quad [6]$$

$$A_1 = \frac{J_H}{2S}\sum_{k,n} f_n(k)\sum_{\alpha,v} v|U^n_{\alpha v}(k)|^2 \quad [7]$$

$$A_2(q) = \frac{{J_H}^2}{2S}\sum_{k,mn}\frac{f_n(k)-f_m(k+q)}{E_n(k)-E_m(k+q)}|\sum_\alpha U^{m*}_{\alpha\downarrow}(k+q)U^n_{\alpha\uparrow}(k)|^2 \quad [8]$$

$$B_2(q) = \frac{{J_H}^2}{2S}\sum_{k,mn}\frac{f_n(k)-f_m(k+q)}{E_n(k)-E_m(k+q)} \times \sum_{\alpha\beta} U^{m*}_{\alpha\downarrow}(k+q)U^n_{\alpha\uparrow}(k)U^{n*}_{\beta\downarrow}(k+q)U^m_{\beta\uparrow}(k) \quad [9]$$

Here diagonal representation $d_{nk}$ of the itinerant Hamiltonian (including the influence of ferro-orbital and anti-ferromagnetic order parameters) is employed $\tilde{c}_{k\alpha v} = \sum_n U^n_{\alpha v}(k)d_{nk}$, with eigenvalue $E_n(k)$ of each band index n. Note that $f_n(k) = 1/(1+e^{\beta(E_n(k)-\mu)})$ denotes the Fermi distribution function with chemical potential $\mu$., which needs to be evaluated for each set of order parameters.

Finally, a simple diagonalization of the spin-wave Hamiltonian gives the spin-wave dispersion

$$\omega(q) = \sqrt{A^2(q) - B^2(q)} \quad [10]$$

and allows an estimation of the fluctuating portion of the moment

$$\Delta m = \frac{1}{8\pi^2}\int dq^2 A(q)/\omega(q) - 1/2 = \frac{1}{8\pi^2}\int dq^2[1-(B_q/A_q)^2]^{-1/2} - 1/2 \quad [11]$$

# III. Some useful numerical tricks

## q-space interpolation

Since the formula to evaluate $\Delta m$ involves integrable singularity, an accurate and very dense mesh of q points is necessary. Making use of the smooth nature of $A_q$ and $B_q$, a useful trick is to evaluate q only in a relatively coarser mesh, say $20 \times 20$ or bigger, and then perform Wannier interpolation to generate a denser mesh, say $20000 \times 20000$ for the computation of $\Delta m$. The simple idea of Wannier interpolation is to Fourier transform $A_q$ and $B_q$ to real space, and enlarges

the size of the periodic boundary condition by filling zeros in the long-range tail, and inverse Fourier transform back to q space. The smoothness of $A_q$ and $B_q$ guarantees the smallness of long-range tail and makes this trick an accurate numerical approximation.

### Special treatment near zero energy when evaluating $\Delta m$

In evaluating $\Delta m$ , one needs to perform the following integration

$$\frac{S}{8\pi^2}\int dq^2 SA(q)/\omega(q) \quad [12]$$

Therefore, special treatment in region of q where the spin wave energy become close to zero. A useful simple trick is to reduce the integration to one-dimension and use semi-analytical approach to treat the small energy region.

$$\frac{S}{8\pi^2}\int dq^2 A(q)/\omega(q) = \int dv\, g^A(v)/v \quad [13]$$

where

$$g^A(v) = \frac{S}{8\pi^2}\int dq^2 A(q)\delta\big(v-\omega(q)\big) \quad [14]$$

is the *A*-weighted density of states. One thus can take the linear coefficient of the expansion of $g^A$ and perform the integration analytically within a small energy range. Caution must be paid though, when the system is close to a phase transition and the linear region of $g^A$ becomes small in energy.

## IV. Band structure and Fermi surface employed in Ref. 21

The very different physical conclusions between our study and that of Ref.21 originate from the different electronic structure of itinerant carriers. Ref. 21 uses a very low filling factor (~0.1), corresponding to a chemical potential $\mu \sim -2.31t_1$, so that there are only two electron pockets in the center of the Brillouin zone, as shown in the figures below (obtained with the same parameters as those in Ref.21.).

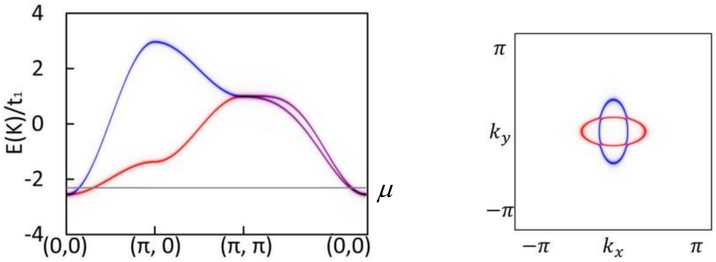

# V. Evolution of Fermi surface and band structure via ferro-orbital order and magnetic order

The figures below compare the effects of ferro-orbital and magnetic order on the band structures and Fermi surfaces.

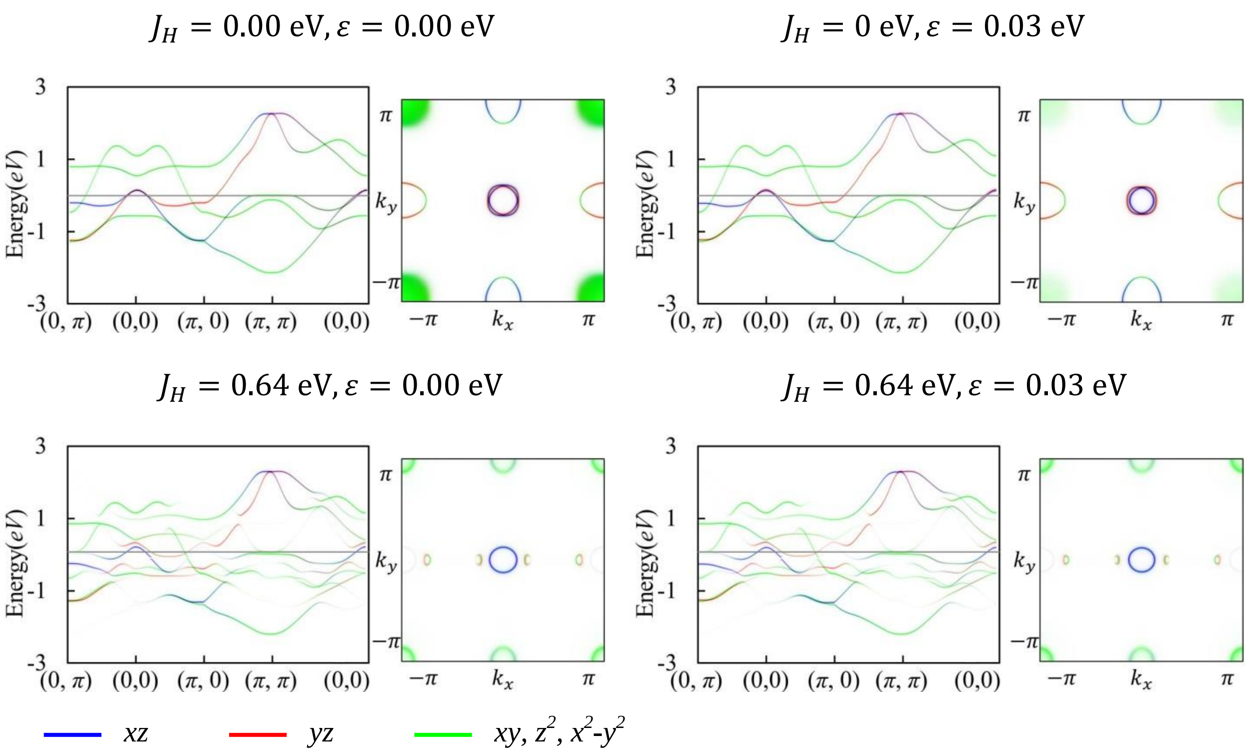


# VI. Insensitivity of qualitative trends against the thermal broadening parameter

Our study considers [Eq.(4)] only the zero-temperature quantum fluctuation $\Delta m$ without thermal fluctuation. The thermal broadening parameter $T$ in the itinerant side is introduced only to ease the numerical calculation. Particularly, we aim at revealing the generic trends in Fe-SCs originated from the approximately nested electron and hole pockets, rather than the material dependence dictated by the details of the Fermi surface. Choosing a larger $T$ thus also helps us avoid being overwhelmed by the details of the Fermi surface of one particular material.

The following figures compare results with two different $T$ parameters (keeping all other parameters identical) and demonstrate clearly the same qualitative trends.

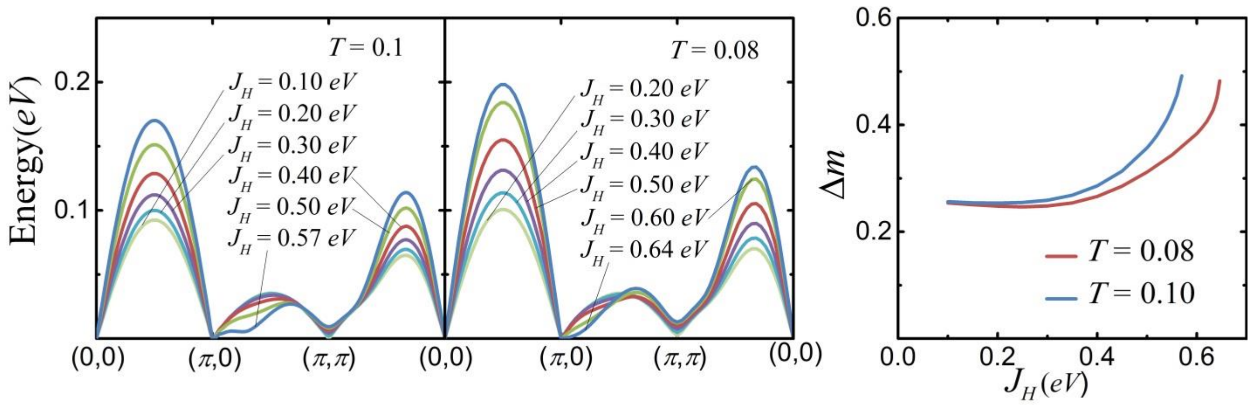


# VII. Other physical considerations

We add here some additional physical consideration that may be considered in future investigations. First, our study focuses on the dominant fluctuation of the local moment, in the spin direction. There in principle should also be weaker fluctuation in the amplitude, since this is an itinerant system. From the phase space argument similar to Pauli vs. Curie susceptibility, one of course would expect such amplitude fluctuation be much weaker at low temperature.

Second, from the separation of local and itinerant degrees of freedom, one should expect that the low-energy bands might not have a full spectral weight of one. The reduced spectral weight should then reduce slightly these bands' contribution to the renormalization, in $A_1$, $A_2$, and $B_2$.

Similarly, one should in principle feed the resulting reduced magnetic order parameter back to the itinerant Hamiltonian, in a self-consistent manner. This would stretch the region of fluctuation to a larger region in the phase diagram, making it more similar to the real materials. The qualitative trends illustrated in the manuscript, however, will remain the same. The last two considerations together can be approximately simulated with a smaller value of $J_H$, as is done in our manuscript.
